# Supplementary material for: SINet: Extreme Lightweight Portrait Segmentation Networks with Spatial Squeeze Modules and Information Blocking Decoder
Source: arXiv:1911.09099 source file (2020-02-09)
Supplement: Supplementary file 2 [file city.tex]

\subsection{Detailed Setting of SINet for Cityscape Dataset}
\label{city}

\begin{table}[ht]

  \begin{center}
      \begin{tabular}{c|c|c|c|c}
          & Input & Operation & Output &  \\
          \hline \hline
    
    1     & $3\times1024\times2048$ & CBR   & $16\times512\times1024$ & Down sampling \\
    2     & $16\times512\times1024$ & DSConv + SE & $\#class\times256\times512$ & Down sampling \\
    3     & $\#class\times256\times512$ & DSConv + SE & $24\times128\times256$ & Down sampling \\
    4     & $24\times128\times256$ & SB module & $60\times128\times256$ & [k=3, p=1], [k=5, p=1] \\
    5     & $60\times128\times256$ & SB module & $60\times128\times256$ & [k=3, p=0], [k=3, p=1] \\
    6     & $60\times128\times256$ & SB module & $60\times128\times256$ & [k=3, p=0], [k=3, p=1] \\
    7     & $84\times128\times256$ & DSConv + SE & $60\times64\times128$ & Concat [3, 6] , Down sampling \\
    8     & $60\times64\times128$ & SB module & $84\times64\times128$ & [k=3, p=1], [k=5, p=1] \\
    9     & $84\times64\times128$ & SB module & $84\times64\times128$ & [k=3, p=0], [k=3, p=1] \\
    10    & $84\times64\times128$ & SB module & $84\times64\times128$ & [k=5, p=1], [k=5, p=4] \\
    11    & $84\times64\times128$ & SB module & $84\times64\times128$ & [k=3, p=2], [k=5, p=8] \\
    12    & $84\times64\times128$ & SB module & $108\times64\times128$ & [k=3, p=1], [k=5, p=1] \\
    13    & $108\times64\times128$ & SB module & $108\times64\times128$ & [k=3, p=1], [k=5, p=1] \\
    14    & $108\times64\times128$ & SB module & $108\times64\times128$ & [k=3, p=0], [k=3, p=1] \\
    15    & $108\times64\times128$ & SB module & $108\times64\times128$ & [k=5, p=1], [k=5, p=8] \\
    16    & $108\times64\times128$ & SB module & $108\times64\times128$ & [k=3, p=2], [k=5, p=4] \\
    17    & $108\times64\times128$ & SB module & $108\times64\times128$ & [k=3, p=0], [k=5, p=2] \\
    18    & $168\times64\times128$ & 1x1 conv & $\#class\times64\times128$ & Concat [7, 17] \\
    
    \end{tabular}%
    \end{center}
    \caption{Detailed setting\Lars{s} for \Lars{the} SINet encoder. k denotes \Lars{the} kernel size of \Lars{the} depthwise convolution and p \Lars{denotes the} kernel size of average pooling \Lars{the} S2-block. }
  \label{tab:citysetting}%
  \vspace{-3mm}
\end{table}%

% Table generated by Excel2LaTeX from sheet 'city_Bench'
\begin{table}[ht]
  \begin{center}

      \begin{tabular}{l | cccccccccc}
    Metric & Average & road  & sidewalk & building & wall  & fence & pole  & trafficlight & trafficsign & vegetation \\
    \hline \hline 
    IoU   & \textbf{66.5}  & 97.4  & 78.9  & 88.9  & 46.6  & 42.7  & 50.5  & 54.3  & 59.9  & 90.8  \\
    iIoU  & 38.3  &   -    & -  &    -    &  -      &  -      &   -     &   -     &   -     &  \\
    \hline 
     Metric     & terrain & sky   & person & rider & car   & truck & bus   & train & motorcycle & bicycle \\
          \hline \hline 
    IoU   & 68.6  & 93.9  & 73.7  & 53.7  & 91.7  & 53.9  & 64.1  & 50.4  & 44.1  & 58.5  \\
    iIoU  &   -     &   -     & 53.5  & 26.8  & 84.7  & 18.8  & 33.1  & 25.3  & 22.3  & 41.8  \\
    \end{tabular}%%
    \end{center}
    \caption{Detailed results on Cityscape testset benchmark}
  \label{tab:citytest}%
  
\end{table}%

Table~\ref{tab:citysetting} is a detailed setting of the encoder model for Cityscape segmentation in the Experiment section. 
The information blocking decoder is used two times with $ 3_{th}$ and $7_{th}$ high-resolution feature maps. 
We used asymmetric depthwise separable convolutions for reducing complexity because we increased the number of layers for handing more complex tasks.
We combined each results of asymmetric depthwise separable convolutions by element-wise summation, and we used original depthwise separable convolution when p is 0.
Table \ref{tab:citytest} is detailed accuracy from Cityscape testset benchmark server.
