# Supplementary material for: SINet: Extreme Lightweight Portrait Segmentation Networks with Spatial Squeeze Modules and Information Blocking Decoder
Source: arXiv:1911.09099 source file (2020-02-09)
Supplement: Supplementary file 3 [file intro.tex]

\section{Supplementary Material}
\label{intro_supp}
In this supplementary material, we provide additional results that we could not include due to space limitations.
First, we report additional latency time result about other input experiments with different dilated rates on an iPhone XS, and another environment(CPU, GPU, NPU) experiments with SINet, MobileNet V3 and ESPNet V2.
Also, we show anther segmentation results.
Second, we indicate another comparison experiment for proving the importance of information blocking with global attention upsampling module \cite{li2018pyramid}.
Finally, we explain a detailed setting of SINet, which is used on a Cityscape experiment.
